# Supplementary material for: Introduction to speech recognition
Source: arXiv:2402.01778 source file (2024-02-01)
Supplement: Supplementary file 3 [file tp0.tex]

\chapter{Travaux pratiques}
